# Supplementary material for: Dominator Coloring and CD Coloring in Almost Cluster Graphs
Source: arXiv:2210.17321 source file (2023-07-29)
Supplement: Supplementary file 1 [file appendix.tex]

% !TEX root = dcoloring.tex
\appendix
\newpage
